# Supplementary material for: Unraveling current-induced dissociation mechanisms in single-molecule junctions
Source: arXiv:2104.05138 source file (2021-05-24)
Supplement: Supplementary file 1 [file Supp_Mat.pdf]

# Supplementary materials for Unraveling current-induced dissociation mechanisms in single-molecule junctions

Yaling Ke,[1] André Erpenbeck,[2] Uri Peskin,[3] and Michael Thoss[1,4]
[1]) *Institute of Physics, Albert-Ludwig University Freiburg, Hermann-Herder-Strasse 3, 79104 Freiburg, Germany*
[2]) *School of Chemistry, The Raymond and Beverley Sackler Center for Computational Molecular and Materials Science, Tel Aviv University, Tel Aviv 6997801, Israel*
[3]) *Schulich Faculty of Chemistry, Technion-Israel Institute of Technology, Haifa 32000, Israel*
[4]) *EUCOR Centre for Quantum Science and Quantum Computing, Albert-Ludwig University Freiburg, Hermann-Herder-Strasse 3, 79104 Freiburg, Germany*

## DERIVATION DETAILS ON THE ELECTRONIC CURRENT EXPRESSION

In this supplementary material, we first provide a detailed derivation on Eq. (38) in the main text, i.e.

$$\begin{aligned} I_\alpha(t) =& -2e\frac{\mathrm{d}}{\mathrm{d}t}\left\langle \sum_k c^\dagger_{\alpha k} c_{\alpha k}\right\rangle \\ =& \frac{2ie}{\hbar}\sum_{l=1}\mathrm{Tr}_s\left\{g_\alpha(Q)\left(d\rho_{\mathbf{0}}^{(\alpha,+,l)}(t) - d^\dagger\rho_{\mathbf{0}}^{(\alpha,-,l)}(t)\right)\right\} \\ &+\frac{2\pi e}{\hbar}\mathrm{Tr}_s\left\{g_\alpha(Q)g_\alpha(Q)\left[dd^\dagger\rho^0_{\mathbf{0}}(t) - d^\dagger d\rho^0_{\mathbf{0}}(t)\right]\right\} \end{aligned} \tag{1}$$

In open quantum system theory, the reduced density matrix is obtained by tracing over all environmental degrees of freedom, $\hat\rho_s(t) = \mathrm{Tr}_{\mathrm{leads+ph}}\{\hat\rho(t)\}$ (to be distinguishable from the variables, the operators are denoted by an overhead hat). As mentioned in the main text, we take the ansatz that the system and the environments are initially factorized and the reservoirs/baths are at their own thermal equilibrium. Due to the Gaussian statistical property of the non-interacting electronic reservoir and the harmonic phonon bath, the reduced density matrix can be expressed explicitly in the Feymann path-integral formalism as[1,2]

$$\begin{aligned} \rho_s(\bar\psi_t,\mathcal{Q}_t,\psi_t,\mathcal{Q}'_t,t) =& \iint \mathrm{d}\bar\psi_i \mathrm{d}\psi_i\int \mathrm{d}\mathcal{Q}_i\int_{\psi_i}^{\bar\psi_t}\mathcal{D}\bar{\boldsymbol\psi}(t)\mathcal{D}\boldsymbol\psi(t)\int_{\mathcal{Q}_i}^{\mathcal{Q}_t}\mathcal{D}\boldsymbol{\mathcal{Q}}(t) \\ &\iint \mathrm{d}\bar\psi'_i \mathrm{d}\psi'_i\int \mathrm{d}\mathcal{Q}'_i\int_{\bar\psi'_i}^{\psi'_t}\mathcal{D}\bar{\boldsymbol\psi}'(t)\mathcal{D}\boldsymbol\psi'(t)\int_{\mathcal{Q}'_i}^{\mathcal{Q}'_t}\mathcal{D}\boldsymbol{\mathcal{Q}}'(t) \\ &e^{\frac{i}{\hbar}S(\bar{\boldsymbol\psi}(t),\boldsymbol\psi(t),\boldsymbol{\mathcal{Q}}(t),\dot{\bar{\boldsymbol\psi}}(t),\dot{\boldsymbol\psi}(t),\dot{\boldsymbol{\mathcal{Q}}}(t),t)}\rho_s(\bar\psi_i,\mathcal{Q}_i,\psi'_i,\mathcal{Q}'_i,0) \\ &e^{-\frac{i}{\hbar}S^*(\bar{\boldsymbol\psi}'(t),\boldsymbol\psi'(t),\boldsymbol{\mathcal{Q}}'(t),\dot{\bar{\boldsymbol\psi}}'(t),\dot{\boldsymbol\psi}'(t),\dot{\boldsymbol{\mathcal{Q}}}'(t),t)}\mathcal{F}(\bar{\boldsymbol\psi}(t),\boldsymbol\psi(t),\boldsymbol{\mathcal{Q}}(t),\bar{\boldsymbol\psi}'(t),\boldsymbol\psi'(t),\boldsymbol{\mathcal{Q}}'(t),t). \end{aligned} \tag{2}$$

Here $\psi$ denotes the eigenvalue of annihilation operator $\hat d$ on a coherent state $|\psi\rangle$, i.e., $\hat d|\psi\rangle = \psi|\psi\rangle$. Its conjugate is $\langle\psi|\hat d^\dagger = \langle\psi|\bar\psi$. $\psi$ and $\bar\psi$ are independent Grassman variables. $\mathcal{Q}$ is the eigenvalue of the nuclear position operator $\hat Q$, $\hat Q|\mathcal{Q}\rangle = \mathcal{Q}|\mathcal{Q}\rangle$, and it is a c-number. $\bar{\boldsymbol\psi}(t)$, $\boldsymbol\psi(t)$, and $\boldsymbol{\mathcal{Q}}(t)$ are forward paths with fixed ending points as specified in the respective integrals. $\bar{\boldsymbol\psi}'(t)$, $\boldsymbol\psi'(t)$, and $\boldsymbol{\mathcal{Q}}'(t)$ are the backward paths. $S$ is the system action functional including the reorganization effect from the thermal bath,

$$\begin{aligned} S(\bar{\boldsymbol\psi}(t),\boldsymbol\psi(t),\boldsymbol{\mathcal{Q}}(t),\dot{\bar{\boldsymbol\psi}}(t),\dot{\boldsymbol\psi}(t),\dot{\boldsymbol{\mathcal{Q}}}(t),t) =& i\hbar\bar{\boldsymbol\psi}(t)\boldsymbol\psi(t) + \int_0^t d\tau\left[-i\hbar\bar{\boldsymbol\psi}(\tau)\dot{\boldsymbol\psi}(\tau) + M\dot{\boldsymbol{\mathcal{Q}}}^2(\tau)/2\right. \\ &- V_g\left(\boldsymbol{\mathcal{Q}}(\tau)\right)\left(1-\bar{\boldsymbol\psi}(\tau)\boldsymbol\psi(\tau)\right) - V_e\left(\boldsymbol{\mathcal{Q}}(\tau)\right)\bar{\boldsymbol\psi}(\tau)\boldsymbol\psi(\tau) \\ &\left.-\lambda f^2(\bar{\boldsymbol\psi}(\tau)\boldsymbol\psi(\tau),\boldsymbol{\mathcal{Q}}(\tau))\right]. \end{aligned} \tag{3}$$

The influence functional $\mathcal{F}$ accounts for the non-Markovian environmental influence on the system dynamics, consisting of the fermionic part for the lead electrons and the bosonic part for the phonons,

$$\begin{aligned} \mathcal{F}(\bar{\boldsymbol\psi}(t),\boldsymbol\psi(t),\boldsymbol{\mathcal{Q}}(t),\bar{\boldsymbol\psi}'(t),\boldsymbol\psi'(t),\boldsymbol{\mathcal{Q}}'(t),t) =& e^{\Phi_{\mathrm{leads}}(\bar{\boldsymbol\psi}(t),\boldsymbol\psi(t),\boldsymbol{\mathcal{Q}}(t),\bar{\boldsymbol\psi}'(t),\boldsymbol\psi'(t),\boldsymbol{\mathcal{Q}}'(t),t)}\times \\ &e^{\Phi_{\mathrm{ph}}(\bar{\boldsymbol\psi}(t),\boldsymbol\psi(t),\boldsymbol{\mathcal{Q}}(t),\bar{\boldsymbol\psi}'(t),\boldsymbol\psi'(t),\boldsymbol{\mathcal{Q}}'(t),t)}, \end{aligned} \tag{4}$$

with the exponents

$$\Phi_{\rm leads} = -\frac{1}{\hbar^2}\sum_{\sigma=\pm,\,\alpha=L/R}\int_0^t {\rm d}\tau\int_0^\tau {\rm d}\tau'\left[\boldsymbol{\psi}^{\bar\sigma}(\tau)g_\alpha\left(\boldsymbol{\mathcal{Q}}(\tau)\right)+\boldsymbol{\psi}'^{\bar\sigma}(\tau)g_\alpha\left(\boldsymbol{\mathcal{Q}}'(\tau)\right)\right]\times \left[C^\sigma_\alpha(\tau-\tau')\boldsymbol{\psi}^{\sigma}(\tau')g_\alpha\left(\boldsymbol{\mathcal{Q}}(\tau')\right)-C^{\bar\sigma *}_\alpha(\tau-\tau')\boldsymbol{\psi}'^{\sigma}(\tau')g_\alpha\left(\boldsymbol{\mathcal{Q}}'(\tau')\right)\right], \tag{5}$$

and

$$\Phi_{\rm ph} = -\frac{1}{\hbar^2}\int_0^t {\rm d}\tau\int_0^\tau {\rm d}\tau'\left[f\left(\bar{\boldsymbol{\psi}}(\tau)\boldsymbol{\psi}(\tau),\boldsymbol{\mathcal{Q}}(\tau)\right)-f\left(\bar{\boldsymbol{\psi}}'(\tau)\boldsymbol{\psi}'(\tau),\boldsymbol{\mathcal{Q}}'(\tau)\right)\right]\times \left[C_{\rm ph}(\tau-\tau')f\left(\bar{\boldsymbol{\psi}}(\tau')\boldsymbol{\psi}(\tau'),\boldsymbol{\mathcal{Q}}(\tau')\right)-C^*_{\rm ph}(\tau-\tau')f\left(\bar{\boldsymbol{\psi}}'(\tau')\boldsymbol{\psi}'(\tau'),\boldsymbol{\mathcal{Q}}'(\tau')\right)\right]. \tag{6}$$

The correlation functions in the above equations are expanded as the sum over exponential functions,

$$C^\sigma_\alpha(t-\tau) = \hbar\pi\delta(t-\tau)+\sum_{l=1}^{L\to\infty}\eta_{\alpha,l}e^{-\gamma^\sigma_{\alpha,l}(t-\tau)}, \tag{7}$$

$$C_{\rm ph}(t-\tau) = \sum_{k=0}^{K}\eta_k e^{-\gamma_k(t-\tau)}+\sum_{k=K+1}^{K\to\infty}\frac{2\eta_k}{\gamma_k}\delta(t-\tau). \tag{8}$$

Substituting Eq. (7) and Eq. (8) into Eq. (5) and Eq. (6), respectively, we can recast the influence functional as

$$\mathcal{F} = e^{\sum_{\sigma=\pm,\,\alpha=L/R}\int_0^t {\rm d}\tau\left[\Theta^\sigma_\alpha(\tau)-\frac{i}{\hbar}\mathcal{A}^{\bar\sigma}_\alpha(\tau)\sum_{l=1}^{\infty}\mathcal{B}^\sigma_{\alpha,l}(\tau)\right]}\cdot e^{\int_0^t {\rm d}\tau\left[\Theta_{ph}(\tau)-\frac{i}{\hbar}\mathcal{A}^{ph}(\tau)\sum_{k=0}^{K}\mathcal{B}^{ph}_k(\tau)\right]}. \tag{9}$$

The expressions for the variables $\{\mathcal{A}\}$, $\{\mathcal{B}\}$, and $\{\Theta\}$ are given by

$$\mathcal{A}^{\bar\sigma}_\alpha(\tau) = \boldsymbol{\psi}^{\bar\sigma}(\tau)g_\alpha\left(\boldsymbol{\mathcal{Q}}(\tau)\right)+\boldsymbol{\psi}'^{\bar\sigma}(\tau)g_\alpha\left(\boldsymbol{\mathcal{Q}}'(\tau)\right), \tag{10}$$

$$\mathcal{A}^{ph}(\tau) = f\left(\bar{\boldsymbol{\psi}}(\tau)\boldsymbol{\psi}(\tau),\boldsymbol{\mathcal{Q}}(\tau)\right)-f\left(\bar{\boldsymbol{\psi}}'(\tau)\boldsymbol{\psi}'(\tau),\boldsymbol{\mathcal{Q}}'(\tau)\right), \tag{11}$$

$$\mathcal{B}^\sigma_{\alpha,l}(\tau) = -\frac{i}{\hbar}\int_0^\tau {\rm d}\tau' e^{-\gamma^\sigma_{\alpha,l}(\tau-\tau')}\left[\eta_{\alpha,l}\boldsymbol{\psi}^{\sigma}(\tau')g_\alpha\left(\boldsymbol{\mathcal{Q}}(\tau')\right)-\eta^*_{\alpha,l}\boldsymbol{\psi}'^{\sigma}(\tau')g_\alpha\left(\boldsymbol{\mathcal{Q}}'(\tau')\right)\right], \tag{12}$$

$$\mathcal{B}^{ph}_k(\tau) = -\frac{i}{\hbar}\int_0^\tau {\rm d}\tau' e^{-\gamma_k(\tau-\tau')}\left[\eta_k f\left(\bar{\boldsymbol{\psi}}(\tau')\boldsymbol{\psi}(\tau'),\boldsymbol{\mathcal{Q}}(\tau')\right)-\eta^*_k f\left(\bar{\boldsymbol{\psi}}'(\tau')\boldsymbol{\psi}'(\tau'),\boldsymbol{\mathcal{Q}}'(\tau')\right)\right], \tag{13}$$

$$\Theta^\sigma_\alpha(\tau) = -\frac{\pi}{2\hbar}\mathcal{A}^{\bar\sigma}_\alpha(\tau)\times\left[\boldsymbol{\psi}^{\sigma}(\tau)g_\alpha\left(\boldsymbol{\mathcal{Q}}(\tau)\right)-\boldsymbol{\psi}'^{\sigma}(\tau)g_\alpha\left(\boldsymbol{\mathcal{Q}}'(\tau)\right)\right], \tag{14}$$

$$\Theta_{ph}(\tau) = -\frac{\tilde{C}_K}{\hbar^2}\mathcal{A}^{ph}(\tau)\times\left[f\left(\bar{\boldsymbol{\psi}}(\tau)\boldsymbol{\psi}(\tau),\boldsymbol{\mathcal{Q}}(\tau)\right)-f\left(\bar{\boldsymbol{\psi}}'(\tau)\boldsymbol{\psi}'(\tau),\boldsymbol{\mathcal{Q}}'(\tau)\right)\right]. \tag{15}$$

Note that $\mathcal{A}^\sigma_\alpha$ and $\mathcal{B}^\sigma_{\alpha,l}$ are Grassman variables obeying the anticommutation relations, for example, $\mathcal{B}^\sigma_{\alpha,l}d^{\bar\sigma} = -d^{\bar\sigma}\mathcal{B}^\sigma_{\alpha,l}$, because they are the linear combination of Grassman variables $\boldsymbol{\psi}^\sigma$, $\boldsymbol{\psi}'^\sigma$ and c-number $g_\alpha(\boldsymbol{\mathcal{Q}})$. $\mathcal{A}_{ph}$ and $\mathcal{B}^{ph}_k$ are c-numbers. Their mutual exchange would not lead to the opposite sign. Based on these variables, one can introduce auxiliary influence functionals,[3,4]

$$\mathcal{F}^{\boldsymbol{n}}_{\boldsymbol{m}} = \frac{1}{\sqrt{\prod_{k=0}^{K}m_k!\,|\eta_k|^{m_k}}}\mathcal{B}_{a_n}\cdots\mathcal{B}_{a_1}(\mathcal{B}^{ph}_K)^{m_K}\cdots(\mathcal{B}^{ph}_0)^{m_0}\mathcal{F} \tag{16}$$

The subscript $\boldsymbol{m}$ is the bosonic index vector $\boldsymbol{m} = (m_0, m_1, \cdots, m_K)$. Every element $m_k$ is a non-negative integer. The superscript $\boldsymbol{n}$ denotes an ordered array of fermionic multi-indices $\boldsymbol{a}_j = (\alpha_j, \sigma_j, l_j)$, i.e., $\boldsymbol{n} = (\boldsymbol{a}_1, \cdots, \boldsymbol{a}_n)$. $\alpha_j$ label the left or right lead. The symbols $\sigma_j$ can be $+$ or $-$, and $l_j$ specify fermionic Padé poles.

By replacing the influence functional $\mathcal{F}$ in the path integral formalism of reduced density matrix $\rho_s$ in Eq. (2) with the auxiliary influence functional $\mathcal{F}_{\boldsymbol{m}}^{\boldsymbol{n}}$, one can readily constitute an extended group of auxiliary density operators, $\{\hat{\rho}_{\boldsymbol{m}}^{\boldsymbol{n}}\}$, and the matrices are given explicitly as

$$\begin{aligned}\rho_{\boldsymbol{m}}^{\boldsymbol{n}}(\bar{\psi}_t, \mathcal{Q}_t, \psi_t, \mathcal{Q}_t', t) = &\iint \mathrm{d}\bar{\psi}_i \mathrm{d}\psi_i \int \mathrm{d}\mathcal{Q}_i \int_{\psi_i}^{\bar{\psi}_t} \mathcal{D}\bar{\boldsymbol{\psi}}(t)\mathcal{D}\boldsymbol{\psi}(t) \int_{\mathcal{Q}_i}^{\mathcal{Q}_t} \mathcal{D}\boldsymbol{\mathcal{Q}}(t) \\ &\iint \mathrm{d}\bar{\psi}_i' \mathrm{d}\psi_i' \int \mathrm{d}\mathcal{Q}_i' \int_{\bar{\psi}_i'}^{\psi_t'} \mathcal{D}\bar{\boldsymbol{\psi}}'(t)\mathcal{D}\boldsymbol{\psi}'(t) \int_{\mathcal{Q}_i'}^{\mathcal{Q}_t'} \mathcal{D}\boldsymbol{\mathcal{Q}}'(t) \\ &e^{\frac{i}{\hbar}S(\bar{\boldsymbol{\psi}}(t),\boldsymbol{\psi}(t),\boldsymbol{\mathcal{Q}}(t),\dot{\bar{\boldsymbol{\psi}}}(t),\dot{\boldsymbol{\psi}}(t),\dot{\boldsymbol{\mathcal{Q}}}(t),t)} \rho_s(\bar{\psi}_i, \mathcal{Q}_i, \psi_i', \mathcal{Q}_i', 0) \\ &e^{-\frac{i}{\hbar}S^*(\bar{\boldsymbol{\psi}}'(t),\boldsymbol{\psi}'(t),\boldsymbol{\mathcal{Q}}'(t),\dot{\bar{\boldsymbol{\psi}}}'(t),\dot{\boldsymbol{\psi}}'(t),\dot{\boldsymbol{\mathcal{Q}}}'(t),t)} \\ &\mathcal{F}_{\boldsymbol{m}}^{\boldsymbol{n}}(\bar{\boldsymbol{\psi}}(t), \boldsymbol{\psi}(t), \boldsymbol{\mathcal{Q}}(t), \bar{\boldsymbol{\psi}}'(t), \boldsymbol{\psi}'(t), \boldsymbol{\mathcal{Q}}'(t), t).\end{aligned} \tag{17}$$

The electronic current between lead $\alpha$ and the molecule is defined as the time derivative of the average number of electron in lead $\alpha$,

$$\begin{aligned}I_\alpha(t) = &-2e\frac{d\langle \hat{N}_\alpha\rangle}{dt} = 2\frac{ie}{\hbar}\mathrm{Tr}\left\{[\hat{N}_\alpha, \hat{H}]\right\} \\ =&2\frac{ie}{\hbar}\mathrm{Tr}\left\{\sum_k g_\alpha(\hat{Q})\left(t_{\alpha k}\hat{c}_{\alpha k}^\dagger \hat{d} - t_{\alpha k}^* \hat{d}^\dagger \hat{c}_{\alpha k}\right)\hat{\rho}(t)\right\} \\ =&2\frac{ie}{\hbar}\mathrm{Tr}_s\left\{-g_\alpha(\hat{Q})\hat{d}\mathrm{Tr}_{\text{leads+ph}}\left\{\sum_k t_{\alpha k}\hat{c}_{\alpha k}^\dagger\hat{\rho}(t)\right\} + g_\alpha(\hat{Q})\hat{d}^\dagger \mathrm{Tr}_{\text{leads+ph}}\left\{\sum_k t_{\alpha k}^*\hat{\rho}(t)\hat{c}_{\alpha k}\right\}\right\}.\end{aligned} \tag{18}$$

To connect the above equation with the auxiliary density matrices, we now express $\mathrm{Tr}_{\text{leads+ph}}\left\{\sum_k t_{\alpha k}\hat{c}_{\alpha k}^\dagger\hat{\rho}(t)\right\}$ in the path-integral formalism

$$\begin{aligned}&\langle \boldsymbol{\psi}_t|\langle \mathcal{Q}_t|\mathrm{Tr}_{\text{leads+ph}}\left\{\sum_k t_{\alpha k}\hat{c}_{\alpha k}^\dagger\hat{\rho}(t)\right\}|\mathcal{Q}_t'\rangle|\boldsymbol{\psi}_t'\rangle \\ =&-\iint \mathrm{d}\bar{\psi}_i \mathrm{d}\psi_i \int \mathrm{d}\mathcal{Q}_i \int_{\psi_i}^{\bar{\psi}_t} \mathcal{D}\bar{\boldsymbol{\psi}}(t)\mathcal{D}\boldsymbol{\psi}(t) \int_{\mathcal{Q}_i}^{\mathcal{Q}_t} \mathcal{D}\boldsymbol{\mathcal{Q}}(t) \iint \mathrm{d}\bar{\psi}_i' \mathrm{d}\psi_i' \int \mathrm{d}\mathcal{Q}_i' \int_{\bar{\psi}_i'}^{\psi_t'} \mathcal{D}\bar{\boldsymbol{\psi}}'(t)\mathcal{D}\boldsymbol{\psi}'(t) \int_{\mathcal{Q}_i'}^{\mathcal{Q}_t'} \mathcal{D}\boldsymbol{\mathcal{Q}}'(t) \\ &e^{\frac{i}{\hbar}S(\bar{\boldsymbol{\psi}}(t),\boldsymbol{\psi}(t),\boldsymbol{\mathcal{Q}}(t),\dot{\bar{\boldsymbol{\psi}}}(t),\dot{\boldsymbol{\psi}}(t),\dot{\boldsymbol{\mathcal{Q}}}(t),t)} \rho_s(\bar{\psi}_i, \mathcal{Q}_i, \psi_i', \mathcal{Q}_i', 0) e^{-\frac{i}{\hbar}S^*(\bar{\boldsymbol{\psi}}'(t),\boldsymbol{\psi}'(t),\boldsymbol{\mathcal{Q}}'(t),\dot{\bar{\boldsymbol{\psi}}}'(t),\dot{\boldsymbol{\psi}}'(t),\dot{\boldsymbol{\mathcal{Q}}}'(t),t)} \\ &\left\{-\frac{i}{\hbar}\int_0^t \left[C_\alpha^+(t-\tau)\bar{\boldsymbol{\psi}}(\tau)g_\alpha\left(\boldsymbol{\mathcal{Q}}(\tau)\right) - C_\alpha^{-*}(t-\tau)\bar{\boldsymbol{\psi}}'(\tau)g_\alpha\left(\boldsymbol{\mathcal{Q}}'(\tau)\right)\right]\mathrm{d}\tau\right\} \\ &\mathcal{F}(\bar{\boldsymbol{\psi}}(t), \boldsymbol{\psi}(t), \boldsymbol{\mathcal{Q}}(t), \bar{\boldsymbol{\psi}}'(t), \boldsymbol{\psi}'(t), \boldsymbol{\mathcal{Q}}'(t), t).\end{aligned} \tag{19}$$

Combining the above equation with Eq. (7), Eq. (12), Eq. (16), and Eq. (17), we can obtain

$$\begin{aligned}&\langle \boldsymbol{\psi}_t|\langle \mathcal{Q}_t|\mathrm{Tr}_{\text{leads+ph}}\left\{\sum_k t_{\alpha k}\hat{c}_{\alpha k}^\dagger\hat{\rho}(t)\right\}|\mathcal{Q}_t'\rangle|\boldsymbol{\psi}_t'\rangle \\ =&\frac{i\pi}{2}g_\alpha(\mathcal{Q}_t)\bar{\psi}_t\rho_s(\bar{\psi}_t, \mathcal{Q}_t, \psi_t, \mathcal{Q}_t', t) - \frac{i\pi}{2}\rho_s(\bar{\psi}_t, \mathcal{Q}_t, \psi_t, \mathcal{Q}_t', t)\bar{\psi}_t' g_\alpha(\mathcal{Q}_t') - \sum_{l=1}\rho_{\boldsymbol{0}}^{(\alpha,+,l)}(\bar{\psi}_t, \mathcal{Q}_t, \psi_t, \mathcal{Q}_t', t).\end{aligned} \tag{20}$$

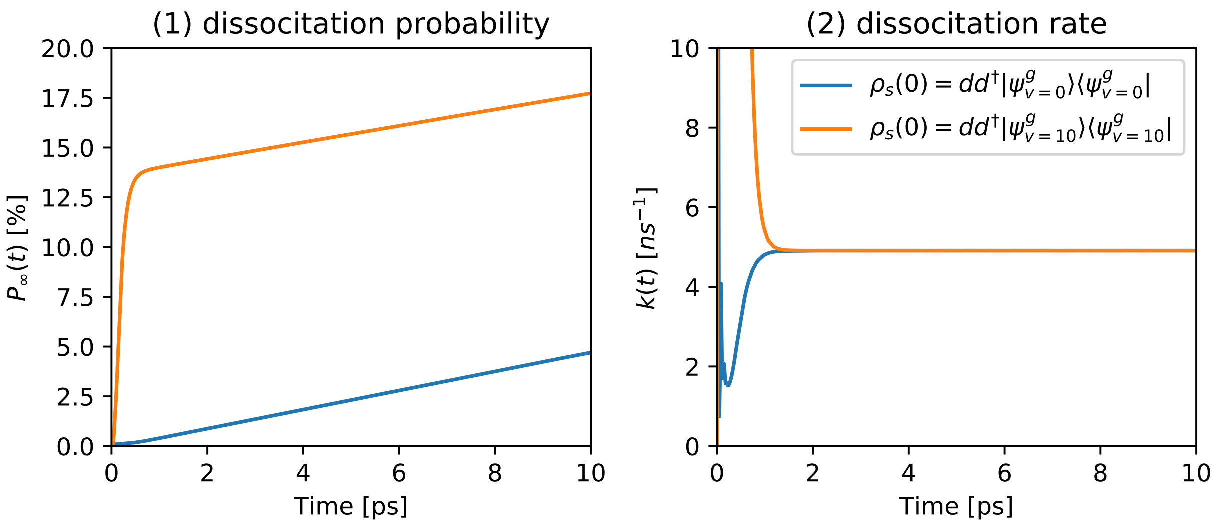


FIG. 1. Time-dependent dissociation probability (1) and rate (2). The blue and orange lines correspond to the results that preparing the initial wavepacket in the ground and the tenth vibrationally excited state, respectively, in the neutral potential surface. Other parameters are: molecule-lead couplings $\Gamma_L = \Gamma_R = 0.05$ eV, the displacement $\Delta Q = 0.3$ Å(c), the bias voltage is $\Phi = 2$ V. The coupling to the secondary phonon bath is neglected.

Similarly, for $\mathrm{Tr}_{\mathrm{leads+ph}}\left\{\sum_k t^*_{\alpha k}\hat{\rho}(t)\hat{c}_{\alpha k}\right\}$, we have

$$\begin{aligned}
&\langle\boldsymbol{\psi}_t|\langle\mathcal{Q}_t|\mathrm{Tr}_r\left\{\hat{\rho}(t)\sum_k t^*_{\alpha k}\hat{c}_{\alpha k}\right\}|\mathcal{Q}'_t\rangle|\boldsymbol{\psi}'_t\rangle\\
=&-\iint \mathrm{d}\bar{\psi}_i\mathrm{d}\psi_i\int\mathrm{d}\mathcal{Q}_i\int_{\psi_i}^{\bar{\psi}_t}\mathcal{D}\bar{\boldsymbol{\psi}}(t)\mathcal{D}\boldsymbol{\psi}(t)\int_{\mathcal{Q}_i}^{\mathcal{Q}_t}\mathcal{D}\boldsymbol{\mathcal{Q}}(t)\iint\mathrm{d}\bar{\psi}'_i\mathrm{d}\psi'_i\int\mathrm{d}\mathcal{Q}'_i\int_{\bar{\psi}'_i}^{\psi'_t}\mathcal{D}\bar{\boldsymbol{\psi}}'(t)\mathcal{D}\boldsymbol{\psi}'(t)\int_{\mathcal{Q}'_i}^{\mathcal{Q}'_t}\mathcal{D}\boldsymbol{\mathcal{Q}}'(t)\\
&e^{\frac{i}{\hbar}S(\bar{\boldsymbol{\psi}}(t),\boldsymbol{\psi}(t),\boldsymbol{\mathcal{Q}}(t),\dot{\bar{\boldsymbol{\psi}}}(t),\dot{\boldsymbol{\psi}}(t),\dot{\boldsymbol{\mathcal{Q}}}(t),t)}\rho_s(\bar{\psi}_i,\mathcal{Q}_i,\psi'_i,\mathcal{Q}'_i,0)e^{-\frac{i}{\hbar}S^*(\bar{\boldsymbol{\psi}}'(t),\boldsymbol{\psi}'(t),\boldsymbol{\mathcal{Q}}'(t),\dot{\bar{\boldsymbol{\psi}}}'(t),\dot{\boldsymbol{\psi}}'(t),\dot{\boldsymbol{\mathcal{Q}}}'(t),t)}\\
&\left\{-\frac{i}{\hbar}\int_0^t\left[C^-_\alpha(t-\tau)\boldsymbol{\psi}(\tau)g_\alpha(\boldsymbol{\mathcal{Q}}(\tau))-C^{+*}_\alpha(t-\tau)\boldsymbol{\psi}'(\tau)g_\alpha\left(\boldsymbol{\mathcal{Q}}'(\tau)\right)\right]\mathrm{d}\tau\right\}\\
&\mathcal{F}(\bar{\boldsymbol{\psi}}(t),\boldsymbol{\psi}(t),\boldsymbol{\mathcal{Q}}(t),\bar{\boldsymbol{\psi}}'(t),\boldsymbol{\psi}'(t),\boldsymbol{\mathcal{Q}}'(t),t)\\
=&\frac{i\pi}{2}g_\alpha(\mathcal{Q}_t)\psi_t\rho_s(\bar{\psi}_t,\mathcal{Q}_t,\psi_t,\mathcal{Q}'_t,t)-\frac{i\pi}{2}\rho_s(\bar{\psi}_t,\mathcal{Q}_t,\psi_t,\mathcal{Q}'_t,t)\psi'_tg_\alpha(\mathcal{Q}'_t)-\sum_{l=1}\rho_{\mathbf{0}}^{(\alpha,-,l)}(\bar{\psi}_t,\mathcal{Q}_t,\psi_t,\mathcal{Q}'_t,t).
\end{aligned}\tag{21}$$

At this point, we can see that

$$\begin{aligned}
I_\alpha(t)=&2\frac{ie}{\hbar}\sum_{l=1}\mathrm{Tr}_s\left\{g_\alpha(\hat{Q})\hat{d}\hat{\rho}_{\mathbf{0}}^{(\alpha,+,l)}(t)-\hat{\rho}_{\mathbf{0}}^{(\alpha,-,l)}(t)\hat{d}^\dagger g_\alpha(\hat{Q})\right\}\\
&+\frac{\pi e}{\hbar}\mathrm{Tr}_s\left\{g_\alpha(\hat{Q})g_\alpha(\hat{Q})\left[\hat{d}\hat{d}^\dagger\rho_{\mathbf{0}}^0(t)-\hat{d}\hat{\rho}_{\mathbf{0}}^0(t)\hat{d}^\dagger-\hat{d}^\dagger\hat{d}\hat{\rho}_{\mathbf{0}}^0(t)+\hat{d}^\dagger\hat{\rho}_{\mathbf{0}}^0(t)\hat{d}\right]\right\}\\
=&2\frac{ie}{\hbar}\sum_{l=1}\mathrm{Tr}_s\left\{g_\alpha(\hat{Q})\hat{d}\hat{\rho}_{\mathbf{0}}^{(\alpha,+,l)}(t)-\hat{\rho}_{\mathbf{0}}^{(\alpha,-,l)}(t)\hat{d}^\dagger g_\alpha(\hat{Q})\right\}\\
&+2\frac{\pi e}{\hbar}\mathrm{Tr}_s\left\{g_\alpha(\hat{Q})g_\alpha(\hat{Q})\left[\hat{d}\hat{d}^\dagger\rho_{\mathbf{0}}^0(t)-\hat{d}^\dagger\hat{d}\hat{\rho}_{\mathbf{0}}^0(t)\right]\right\}
\end{aligned}\tag{22}$$

## INFLUENCE OF THE INITIAL STATE ON THE DYNAMICS

In this part, we compare the dynamics for two different initial states. Fig. 1 displays the time-dependent dissociation probability $P_\infty(t)$ and transient dissociation rate ($k(t)=\frac{d\ln(1-P_\infty(t))}{dt}$). Fig. 2 shows the population dynamics of the vibronic states. The initial state has a substantial impact on the initial dissociation probability and short-time dynamics. The initial dissociation probability can be as high as about 13% if one prepares the initial wavepacket in

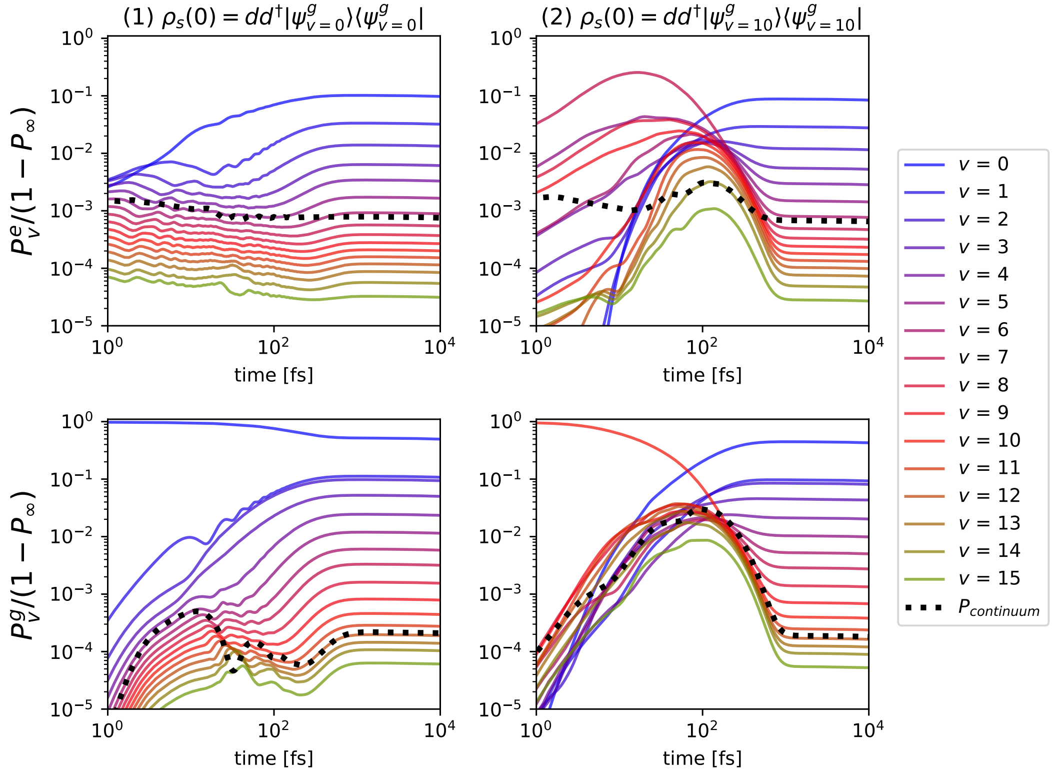


FIG. 2. Population dynamics for different initial states: (1) the vibrational ground state and (2) the tenth vibrationally excited state. The upper and lower panel correspond to the charged and neutral state, respectively. In each panel, the renormalized populations of vibrational bound states are shown as color solid lines and the summation over the populations of the continuum states is shown in black dotted lines. Other parameters are: molecule-lead couplings $\Gamma_L = \Gamma_R = 0.05$ eV, the displacement $\Delta Q = 0.3$ Å(c), the bias voltage is $\Phi = 2$ V. The coupling to the secondary phonon bath is neglected.

the tenth vibrationally excited state in the neutral potential surface. Nevertheless, the long-time dynamics (governed by dissociation rate) and the rescaled quasi-steady vibronic distribution are the same for both initial states.


[1]R. P. Feynman, A. R. Hibbs, and D. F. Styer, *Quantum mechanics and path integrals* (Courier Corporation, 2010).

[2]J. Zinn-Justin, *Quantum field theory and critical phenomena*, Vol. 113 (Clarendon Press, Oxford, 2002).

[3]J. Jin, X. Zheng, and Y. Yan, "Exact dynamics of dissipative electronic systems and quantum transport: Hierarchical equations of motion approach," J. Chem. Phys. **128**, 234703 (2008).

[4]Q. Shi, L. Chen, G. Nan, R.-X. Xu, and Y. Yan, "Efficient hierarchical liouville space propagator to quantum dissipative dynamics," J. Chem. Phys. **130**, 084105 (2009).
